# Supplementary material for: JAX FDM: A differentiable solver for inverse form-finding
Source: arXiv:2307.12407 source file (2023-10-29)
Supplement: Supplementary file 1 [file appendix.tex]

\newpage
\appendix
\onecolumn
\section{You \emph{can} have an appendix here.}

You can have as much text here as you want. The main body must be at most $8$ pages long.
For the final version, one more page can be added.
If you want, you can use an appendix like this one, even using the one-column format.
